# Supplementary material for: Multiple Hypothesis Flow Estimation for Video Frame Interpolation under Matching Ambiguity
Source: arXiv:2608.07120 source file (2026-11-27)
Supplement: Supplementary file 1 [file X_suppl.tex]

\clearpage
\setcounter{page}{1}
\maketitlesupplementary



\begin{figure*}[!t]
    \centering
    \includegraphics[width=0.95\textwidth]{SM1.png}
\caption{
Qualitative comparison with generative VFI approaches on challenging
examples, involving dynamic textures, particle-like motion,
rotational symmetry, thin structures, fast motion, and partial
occlusion.
From left to right, the figure presents two visualizations of the input-frame motion (a semi-transparent overlay and a red–cyan anaglyph), followed by results from our method, PerVFI, TLB-VFI, and LDMVFI.
The input overlays provide
a visual indication of inter-frame motion and matching difficulty.
Across these examples, our method preserves sharper local structures
and more coherent object geometry. These qualitative observations are
consistent with the corresponding LPIPS and DISTS results. Best viewed enlarged.
}
\label{fig:generative-vfi}
\end{figure*}
\section*{Results on Vimeo90K}
\label{sec:supp-vimeo90k}

We further evaluate the complete model on the standard Vimeo90K~\cite{xue2019video} test
set to examine whether its performance remains competitive beyond the
curated matching-ambiguity scenarios in MA-HD. Quantitative
comparisons with recent state-of-the-art methods are summarized in
Table~\ref{tab:vimeo90k}.

Our method achieves the best LPIPS and DISTS scores among the compared
approaches (\textbf{1.92} and \textbf{2.01}, respectively, both
scaled by $\times100$), while obtaining a PSNR of
\textbf{35.68}\,dB. These results show that the perceptual advantage
of the complete model is not restricted to MA-HD and remains visible
on a standard general-purpose VFI benchmark. Because this comparison
evaluates complete systems rather than a same-recipe $K=1$ control,
we do not attribute the entire gain solely to the multi-hypothesis
component.

In terms of computational cost, our method uses \textbf{3.54}\,GB of GPU memory and runs at
\textbf{1.71}\,FPS under the evaluation setting reported in Table~\ref{tab:vimeo90k}.



\begin{table}[ht]
\centering
\setlength{\tabcolsep}{4pt} % 收紧列间距，原版默认6pt
\small
\sisetup{
  detect-weight=true,
  detect-inline-weight=math,
  table-align-text-pre=false,
  table-align-text-post=false
}
\begin{tabular}{@{}l
  S[table-format=2.2]
  S[table-format=2.2]
  S[table-format=2.2]
  S[table-format=2.2]
  S[table-format=1.2]
  @{}}
\toprule
Method & {LPIPS$\downarrow$} & {DISTS$\downarrow$} & {PSNR$\uparrow$} & {Mem$\downarrow$ (GB)} & {FPS$\uparrow$} \\
\midrule
EMA-VFI   & 2.64 & 2.38 & \bfseries 36.64 & 7.87 & 1.54 \\
SGM-VFI   & 3.24 & 3.09 & 34.96 & \underline{3.75}  & 1.58  \\
PerVFI    & 2.87 & \underline{2.04} & 33.89 & 6.85 & 1.33 \\
AMT-G     & \underline{2.58} & 2.69 & \underline{36.53} & 4.99 & \bfseries 2.88 \\
LC-Mamba  & 3.80 & 3.74 & 36.43 & 26.16 & 1.30 \\
\midrule
\textbf{Ours} & \bfseries 1.92 & \bfseries 2.01 & 35.68 & \bfseries 3.54 & \underline{1.71} \\
\bottomrule
\end{tabular}
\caption{Quantitative comparison on Vimeo90K benchmark. LPIPS and DISTS are scaled by $\times100$. Memory is the peak per-GPU usage in GB on a single NVIDIA A100 with batch
size 1; FPS is the overall average frame rate. Best and second-best in each column are \textbf{bold}
and \underline{underlined}.}
\vspace{-6pt}
\label{tab:vimeo90k}
\end{table}

\section*{Comparison with Generative VFI Methods}
\label{sec:supp-generative-comparison}

\begin{figure*}[ht]
    \centering
    \includegraphics[width=\textwidth]{data.png}
    \caption{
    Representative examples of the training-time augmentations.
    From top to bottom, the rows show the unaugmented triplets, additive
    Gaussian noise, photometric jitter, horizontal flipping, spatial
    rescaling, and motion blur. Within each example group, the columns
    correspond to the first endpoint frame, the ground-truth middle
    frame, and the second endpoint frame.
    }
    \label{fig:augmentation-examples}
\end{figure*}

We further compare our method with three representative generative VFI
approaches on SNU-FILM~\cite{choi2020channel}: PerVFI~\cite{Wu_2024_CVPR}, which performs conditional frame
generation, and TLB-VFI~\cite{lyu2025tlb} and LDMVFI~\cite{danier2024ldmvfi}, which employ diffusion-based
generation. The quantitative results across the four difficulty levels
are reported in Table~\ref{tab:generative-vfi}, while representative
visual comparisons are provided in Fig.~\ref{fig:generative-vfi}.

\begin{table*}[htbp!]
\centering
\small
\setlength{\tabcolsep}{5.0pt}

\begin{tabular}{@{}lcccccccccccc@{}}
\toprule
& \multicolumn{3}{c}{Easy}
& \multicolumn{3}{c}{Medium}
& \multicolumn{3}{c}{Hard}
& \multicolumn{3}{c}{Extreme} \\
\cmidrule(lr){2-4}
\cmidrule(lr){5-7}
\cmidrule(lr){8-10}
\cmidrule(lr){11-13}
Method
& LPIPS$\downarrow$ & DISTS$\downarrow$ & PSNR$\uparrow$
& LPIPS$\downarrow$ & DISTS$\downarrow$ & PSNR$\uparrow$
& LPIPS$\downarrow$ & DISTS$\downarrow$ & PSNR$\uparrow$
& LPIPS$\downarrow$ & DISTS$\downarrow$ & PSNR$\uparrow$ \\
\midrule
TLB-VFI
& \textbf{1.20} & \textbf{0.92} & \underline{39.46}
& \textbf{2.10} & \textbf{1.45} & \textbf{35.31}
& \underline{4.40} & 2.78 & 29.53
& 9.50 & 4.89 & 24.51 \\

LDMVFI
& \underline{1.40} & \underline{1.07} & 38.67
& \underline{2.80} & \underline{1.93} & 34.00
& 6.00 & 3.80 & 28.55
& 12.30 & 6.33 & 23.93 \\

PerVFI
& 2.02 & 1.53 & 38.44
& 2.95 & 2.10 & \underline{34.80}
& 4.71 & \underline{2.76} & \underline{29.92}
& \underline{9.02} & \underline{4.48} & \underline{25.07} \\
\midrule

\textbf{Ours}
& 1.95 & 1.49 & \textbf{39.72}
& 2.83 & 1.95 & 34.56
& \textbf{4.22} & \textbf{2.67} & \textbf{31.12}
& \textbf{7.79} & \textbf{4.01} & \textbf{26.26} \\
\bottomrule
\end{tabular}
\caption{
Quantitative comparison with generative VFI methods on the four
difficulty levels of SNU-FILM. LPIPS and DISTS are scaled by $\times100$.
The best and second-best results in each column are shown in
\textbf{bold} and \underline{underlined}, respectively.
}
\label{tab:generative-vfi}
\end{table*}



Among the generative VFI methods considered in
Table~\ref{tab:generative-vfi}, the diffusion-based methods
achieve lower LPIPS and DISTS on the Easy subset, whereas
our method obtains the highest PSNR of 39.72\,dB.
On the Medium subset, TLB-VFI achieves the best results
across all three metrics, with an LPIPS of $2.10$,
a DISTS of $1.45$, and a PSNR of $35.31$\,dB.
Our perceptual scores (LPIPS $2.83$ and DISTS $1.95$)
remain close to those of LDMVFI ($2.80$ and $1.93$,
respectively) and PerVFI ($2.95$ and $2.10$,
respectively).

As the interpolation difficulty increases, our method
demonstrates a clearer performance advantage.
On both the Hard and Extreme subsets, our method
achieves the best LPIPS, DISTS, and PSNR among the
compared approaches.
On the Hard subset, it improves the best competing
results from $4.40$ to $4.22$ in LPIPS, from $2.76$
to $2.67$ in DISTS, and from $29.92$ to $31.12$\,dB
in PSNR.
On the Extreme subset, the improvements become more
pronounced: our method reduces LPIPS from $9.02$
to $7.79$ (a relative reduction of approximately
$13.6\%$) and DISTS from $4.48$ to $4.01$
(a relative reduction of approximately $10.5\%$),
while increasing PSNR from $25.07$ to $26.26$\,dB.

These comparisons evaluate complete systems rather
than controlled variants with identical training
recipes. Therefore, the observed performance differences
cannot be attributed solely to the generative paradigm
or the proposed multi-hypothesis formulation, as they
may also depend on motion representation, training data,
reconstruction objectives, and model capacity.
Nevertheless, the results demonstrate that the proposed
correspondence-conditioned formulation remains
competitive with generative VFI approaches and provides
stronger perceptual fidelity on the more difficult
SNU-FILM subsets.



As illustrated in Fig.~\ref{fig:generative-vfi}, the quantitative
advantage on the Hard and Extreme subsets is also reflected in the
qualitative examples. In the dynamic-texture and particle cases, our
method retains more visible high-frequency structure. In the
windmill, tree-branch, and bicycle examples, it produces more coherent
geometry and fewer fragmented structures. These observations are
consistent with the quantitative LPIPS and DISTS results, although
they should not be interpreted as direct evidence of physical motion
accuracy.


\begin{table*}[htbp!]
\centering
\normalsize
\setlength{\tabcolsep}{6pt}
\begin{tabular}{@{}lcccccc@{}}
\toprule
& \multicolumn{3}{c}{Hard}
& \multicolumn{3}{c}{Extreme} \\
\cmidrule(lr){2-4}\cmidrule(lr){5-7}
Training recipe
& LPIPS$\downarrow$ & DISTS$\downarrow$ & PSNR$\uparrow$
& LPIPS$\downarrow$ & DISTS$\downarrow$ & PSNR$\uparrow$ \\
\midrule
Ours (w/o augmentation)
& 5.02 & 3.24 & 30.45
& 9.14 & 4.88 & 25.45 \\
Ours (Group A only)
& 4.55 & 2.91 & 30.89
& 8.22 & 4.30 & 25.97 \\
Ours (Group B only)
& 4.73 & 3.02 & 30.72
& 8.51 & 4.43 & 25.78 \\
Ours (Full augmentation)
& \textbf{4.22} & \textbf{2.67} & \textbf{31.12}
& \textbf{7.79} & \textbf{4.01} & \textbf{26.26} \\
\bottomrule
\end{tabular}
\caption{
Ablation study of grouped training augmentations on the Hard and Extreme subsets of SNU-FILM.
Group A denotes spatial-geometric augmentations (random horizontal flipping and large-scale spatial rescaling),
while Group B denotes pixel- and image-quality augmentations (additive Gaussian noise, mild photometric jitter, and motion blur).
The ``Ours (w/o augmentation)'' setting denotes the baseline without either augmentation group.
``Ours (Group A only)'' and ``Ours (Group B only)'' enable only the corresponding augmentation group, respectively.
``Ours (Full augmentation)'' combines both groups and corresponds to the full augmentation configuration used in the main paper.
LPIPS and DISTS are scaled by $\times 100$.
}
\label{tab:grouped-augmentation-ablation}
\end{table*}

\section*{Data Augmentation}
\label{sec:supp-data-augmentation}

We augment the Vimeo90K training triplets with additive Gaussian
noise, mild photometric jitter, random horizontal flipping,
large-scale spatial rescaling, and motion blur. The geometric
transformations are applied consistently to the input and target
frames of each triplet so that their spatial correspondence is
preserved. Gaussian noise and photometric jitter improve robustness
to low-level appearance perturbations, while spatial rescaling and
motion blur expose the model to larger apparent displacement and
degraded matching evidence.

Figure~\ref{fig:augmentation-examples} visualizes representative
training triplets before and after applying each augmentation type.
Each three-column group contains the two endpoint frames and the
corresponding ground-truth middle frame. The examples are included to illustrate the visual effect of the augmentation operators; they are not used as quantitative evidence.

We divide the training augmentations into two groups according to the
type of variation they introduce. Group A contains spatial-geometric
augmentations, including random horizontal flipping and large-scale
spatial rescaling. Group B contains pixel- and image-quality
augmentations, including additive Gaussian noise, mild photometric
jitter, and motion blur. We evaluate the baseline without either group,
with each group separately, and with both groups enabled. All variants
use the same architecture, losses, optimizer, learning-rate schedule,
training data, and number of training epochs; only the augmentation
configuration is changed.


The trend suggests that both augmentation groups may improve
robustness on difficult interpolation cases, with spatial-geometric
augmentation expected to contribute more strongly under large motion
and the combined recipe expected to perform best.

As shown in Table~\ref{tab:grouped-augmentation-ablation}, both augmentation groups improve the interpolation performance on the challenging Hard and Extreme subsets. Spatial-geometric augmentations (Group A) provide larger individual gains than pixel- and image-quality augmentations (Group B), while combining both groups achieves the best overall performance.
